# Supplementary material for: Accurate complex-stacking-fault Gibbs energy in Ni3Al at high temperatures
Source: arXiv:2508.15528 source file (2025-08-21)
Supplement: Supplementary file 1 [file CSF_supplementary.pdf]

# Supplementary Information to “Accurate temperature-dependent complex-stacking-fault Gibbs energy in $\text{Ni}_3\text{Al}$ ”

Xiang Xu<sup>1,2</sup>, Xi Zhang<sup>2\*</sup>, Andrei Ruban<sup>3,4</sup>, Siegfried Schmauder<sup>1</sup>, and Blazej Grabowski<sup>2</sup>

<sup>1</sup>*Institute for Materials Testing, Materials Science and Strength of Materials, University of Stuttgart, Pfaffenwaldring 32, 70569 Stuttgart, Germany*

<sup>2</sup>*Institute for Materials Science, University of Stuttgart, Pfaffenwaldring 55, 70569 Stuttgart, Germany*

<sup>3</sup>*KTH Royal Institute of Technology, SE-100 44 Stockholm, Sweden*

<sup>4</sup>*Materials Center Leoben Forschung GmbH, A-8700 Leoben, Austria*

\*Corresponding author: xi.zhang@imw.uni-stuttgart.de

## Supp. 1 eDOS

Figure S1 and S2 show the partial electronic density of states of Ni atoms in bulk  $\text{Ni}_3\text{Al}$  and in the CSF structure (the tilted cell in Figure 2 in the main text) at zero-Kelvin. The influence of inserting a CSF plane decays when departing from the CSF plane and almost vanishes when  $l = 3$ , confirming that a model with six atomic layers is sufficient to exclude the interaction between the CSF and its periodic images.

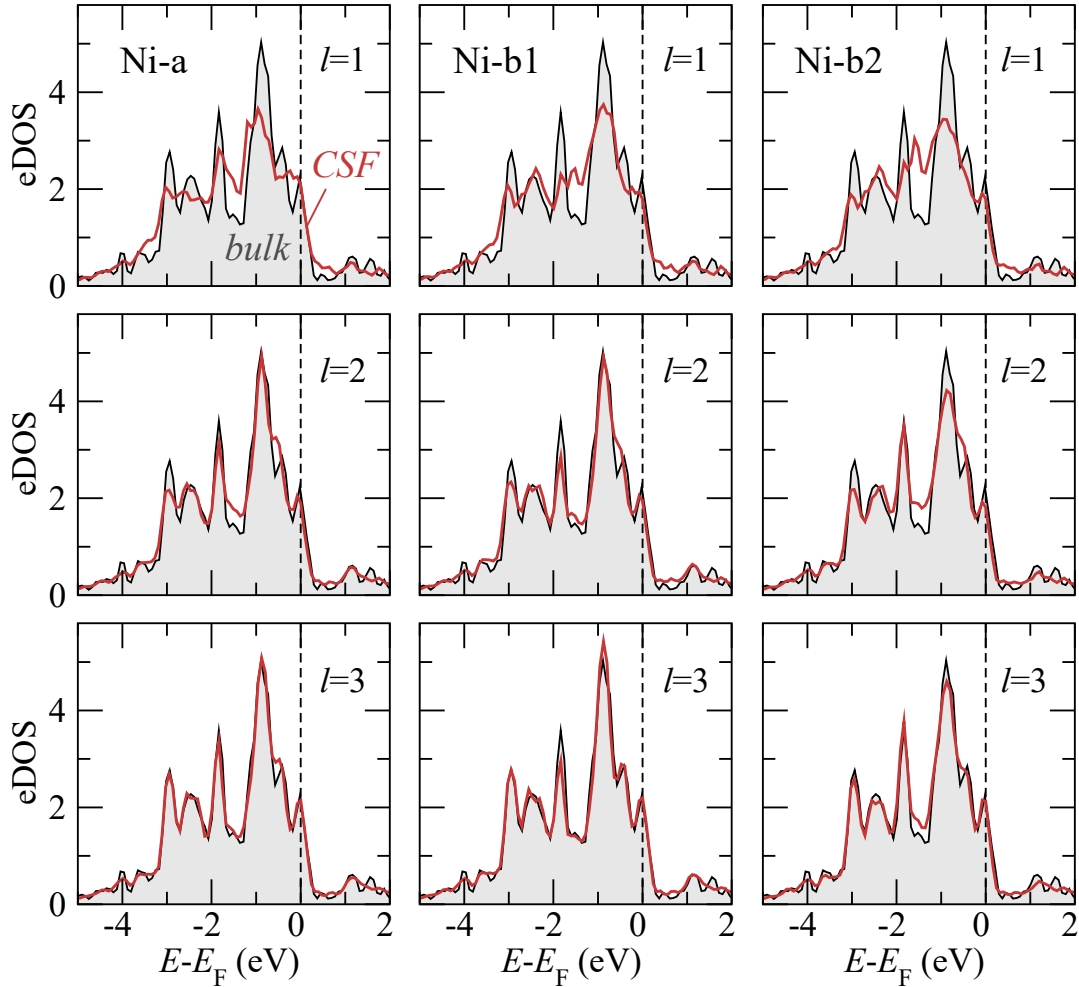

Figure S1: Partial electronic density of states (eDOS) for Ni atoms in the CSF structure and bulk  $\text{Ni}_3\text{Al}$  from spin-unpolarized calculations.  $E_F$  refers to the Fermi energy. The value of  $l$  gives the distance to the CSF in terms of atomic layers. Each atomic layer has three Ni atoms labeled as "Ni-a", "Ni-b1" and "Ni-b2" ("Ni-b1" and "Ni-b2" are equivalent).

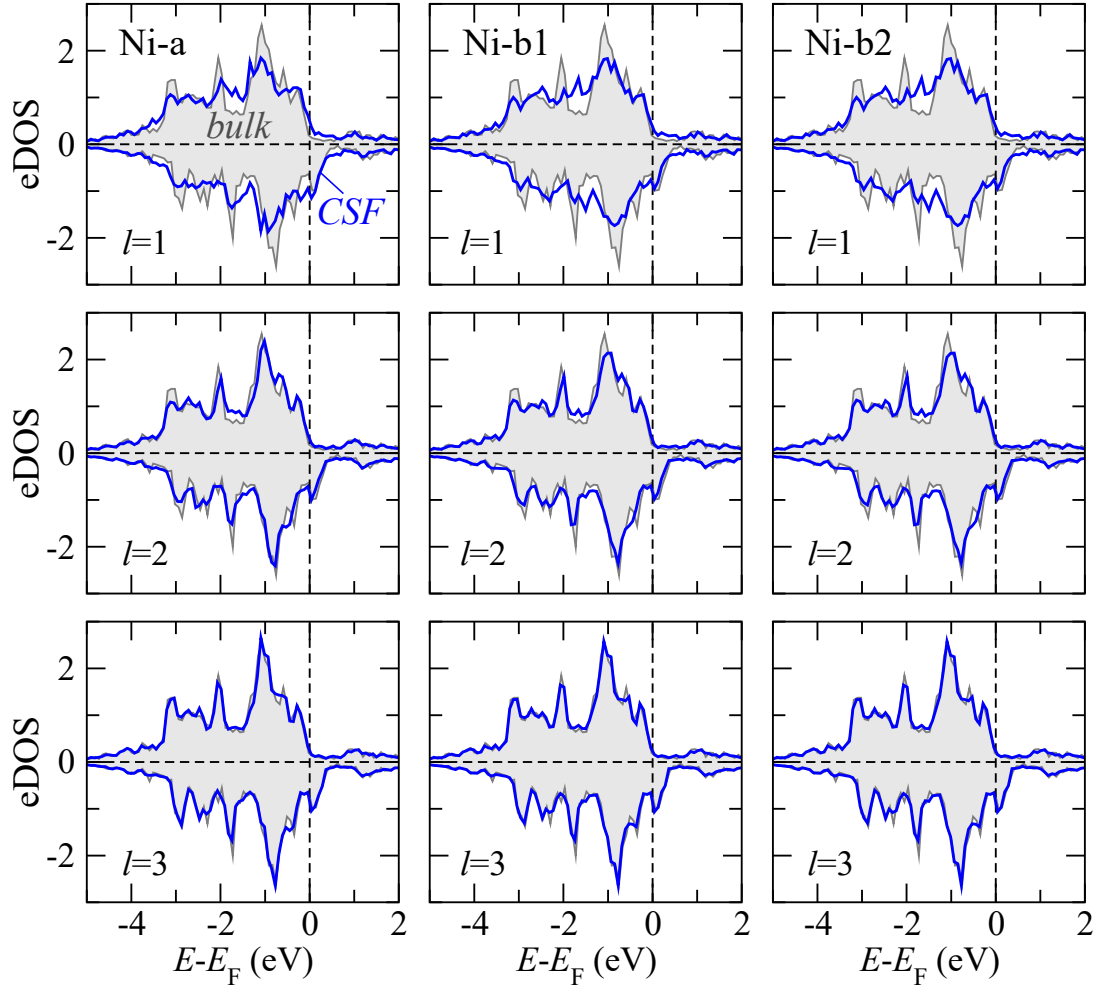

Figure S2: Partial electronic density of states (eDOS) for Ni atoms in the CSF structure and bulk  $\text{Ni}_3\text{Al}$  from spin-polarized calculations.

## Supp. 2 Distribution of Pair Interactions

Distributions of several millions of atomic pairs are collected from MD simulations with using the Langevin dynamics with the fitted MTP. Here, the trained MTP was utilized, which ensures the accuracy and efficiency of the vibrational phase space. When including the anharmonicity, the first nearest-neighbor (1NN) pair distribution shows a typical wall-like planar edge [1, 2], while the quasiharmonic distribution is symmetric, as shown in Figure S3. It is interesting that the in-plane 1NN pair interactions demonstrate similar distributions for both bulk and CSF structures. The anharmonic term in Equation (2) in the main text can be characterized by the difference between the full-vibration distribution and the QH-vibration distribution.

On the other hand, the cross-plane 1NN distributions present an evident deviation between bulk and CSF structures, as shown in Figure S4. This difference is assumed to be the reason for the substantial anharmonic contribution to the CSF energy at higher temperatures.

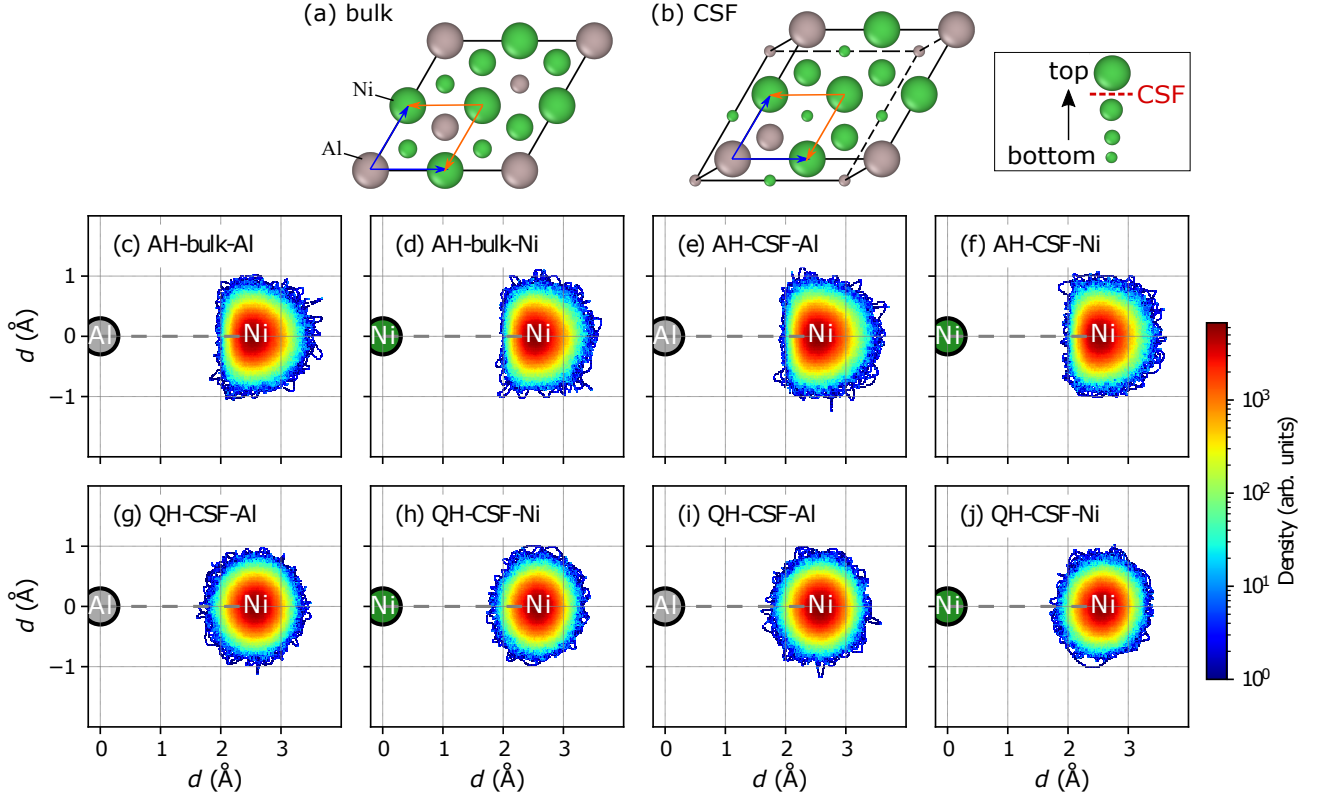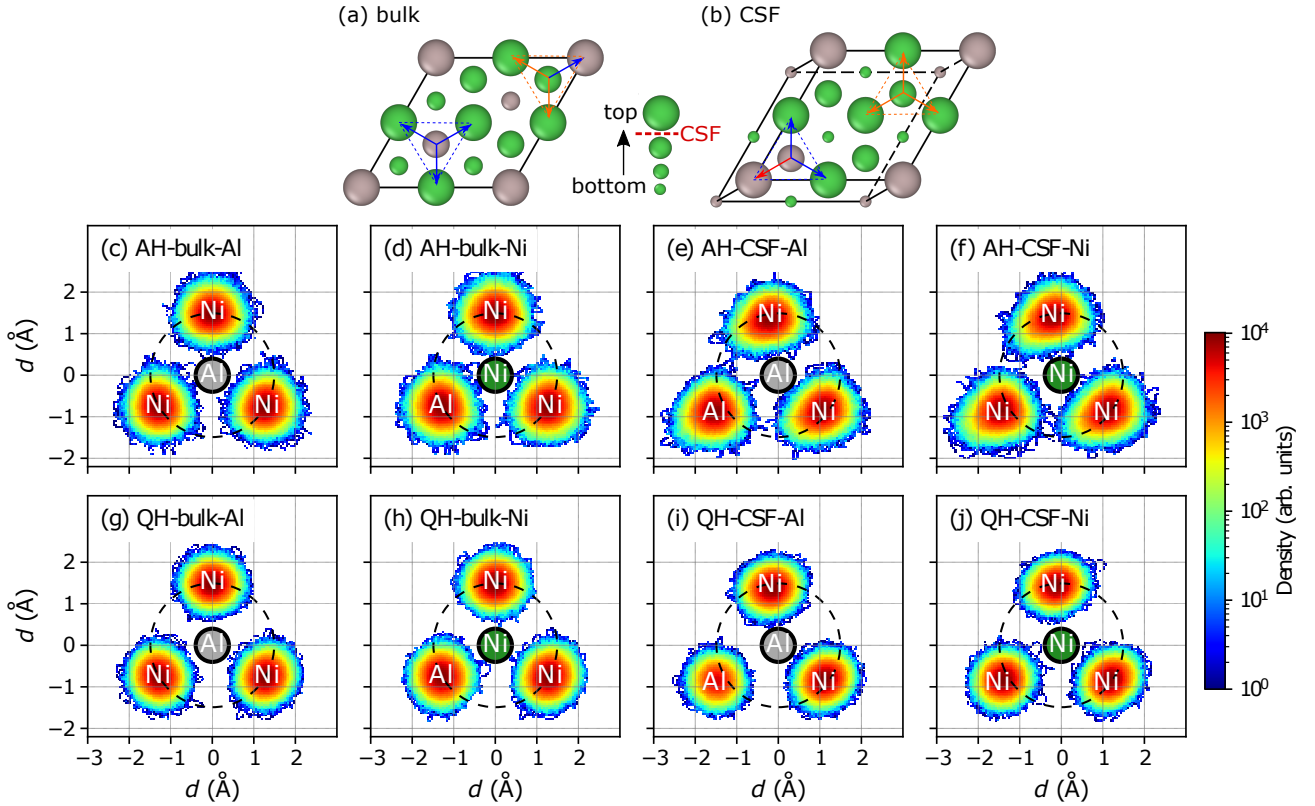

Figure S4: Cross-plane distributions in  $\text{Ni}_3\text{Al}$  and CSF structures at 1454 K and at the corresponding equilibrium lattice constant of 3.65 Å. (a) (d) The atomic positions projected onto the (111) plane. Blue, orange and red arrows indicate the Al-Ni, Ni-Ni and Al-Al pairs, respectively. (c) to (d) are the distribution considering full vibrations, while (g) to (j) are only from quasi-harmonic force constants. Dashed black circles represent the 1NN distance at a lattice constant of 3.65 Å in bulk  $\text{Ni}_3\text{Al}$ .

## Supp. 3 Collection of CSF energies

Table S1: Collection of CSF energies in  $\text{mJ}/\text{m}^2$ . Experimental values marked with “†” are shown in Figure 3 in the main text. RT: room temperature. EAM: Embedded Atom Model; TB-LMTO: Tight Binding Linear Muffin-Tin Orbitals; FLMT0-PN: Full-Potential Linear Muffin-Tin Orbital within the Peierls–Nabarro model.

| Experiments                                                |                                                   |                                     |                |
|------------------------------------------------------------|---------------------------------------------------|-------------------------------------|----------------|
| Reference                                                  | Composition                                       | Energies ( $\text{mJ}/\text{m}^2$ ) | $T$ (K)        |
| Hemker1993 [3]                                             | $\text{Ni}_{76}\text{Al}_{24}$                    | $206 \pm 30$                        | 485            |
| Karnthaler1996 [4]                                         | $\text{Ni}_{78}\text{Al}_{22}$                    | $235 \pm 40$                        | RT             |
| Kruml2002 [5]                                              | $\text{Ni}_{76}\text{Al}_{24}$                    | $206 \pm 27$                        | RT             |
| Kruml2002 [5]                                              | $\text{Ni}_{75}\text{Al}_{25}$                    | $236 \pm 29$                        | RT             |
| Kruml2002 [5]                                              | $\text{Ni}_{74}\text{Al}_{26}$                    | $277 \pm 49$                        | RT             |
| Baluc1991 [6]                                              | $\text{Ni}_{74.3}\text{Al}_{24.7}\text{Ta}_{1.0}$ | $300 \pm 40$                        | RT             |
| Hemker1993 [3]                                             | $\text{Ni}_{75.5}\text{Al}_{23.8}\text{B}_{0.7}$  | $335 \pm 60$                        | 485            |
| Theoretical calculations at 0 K for $\text{Ni}_3\text{Al}$ |                                                   |                                     |                |
| Reference                                                  | Method                                            | Energies ( $\text{mJ}/\text{m}^2$ ) | Magnetic state |
| <i>present work</i>                                        | DFT, PAW-PBE                                      | 217                                 | FM             |
| <i>present work</i>                                        | DFT, PAW-PBE                                      | 171                                 | NM             |
| Rosengaard1994 [7]                                         | DFT, TB-LMTO                                      | 308                                 | FM             |
| Mryasov2002 [8]                                            | DFT, FLMT0-PN                                     | 225                                 |                |
| Yu2012 [9]                                                 | DFT, PAW-PBE                                      | 202                                 | FM             |
| Liu2015 [10]                                               | DFT, PAW-PBE                                      | 208                                 | FM             |
| Rao2018 [11]                                               | DFT, PAW-PW91                                     | 187                                 | FM             |
| Mishin2004 [12]                                            | EAM                                               | 202                                 |                |
| Chen1989 [13]                                              | EAM                                               | 120                                 |                |
| Du2012 [14]                                                | EAM                                               | 218                                 |                |

## References

- [1] A. Glensk, B. Grabowski, T. Hickel, and J. Neugebauer. Understanding anharmonicity in fcc materials: From its origin to *ab initio* strategies beyond the quasiharmonic approximation. *Physical review letters*, 114(19):195901, 2015. doi: [10.1103/PhysRevLett.114.195901](https://doi.org/10.1103/PhysRevLett.114.195901).
- [2] P. Srinivasan, A. Shapeev, J. Neugebauer, F. Körmann, and B. Grabowski. Anharmonicity in bcc refractory elements: A detailed *ab initio* analysis. *Physical Review B*, 107(1):014301, 2023. doi: [10.1103/PhysRevB.107.014301](https://doi.org/10.1103/PhysRevB.107.014301).
- [3] K. J. Hemker and M. J. Mills. Measurements of antiphase boundary and complex stacking fault energies in binary and B-doped  $\text{Ni}_3\text{Al}$  using TEM. *Philosophical Magazine A*, 68(2):305–324, 1993. doi: [10.1080/01418619308221207](https://doi.org/10.1080/01418619308221207).
- [4] H. P. Karnthaler, E. Th. Mühlbacher, and C. Rentenberger. The influence of the fault energies on the anomalous mechanical behaviour of  $\text{Ni}_3\text{Al}$  alloys. *Acta Materialia*, 44(2):547–560, 1996. doi: [10.1016/1359-6454\(95\)00191-3](https://doi.org/10.1016/1359-6454(95)00191-3).
- [5] T. Kruml, E. Conforto, B. Lo. Piccolo, D. Caillard, and J. L. Martin. From dislocation cores to strength and work-hardening: a study of binary  $\text{Ni}_3\text{Al}$ . *Acta materialia*, 50(20):5091–5101, 2002. doi: [10.1016/S1359-6454\(02\)00364-6](https://doi.org/10.1016/S1359-6454(02)00364-6).
- [6] N. Baluc, H. P. Karnthaler, and M. J. Mills. TEM observation of the fourfold dissociation of superlattice dislocations and the determination of the fault energies in  $\text{Ni}_3(\text{Al}, \text{Ta})$ . *Philosophical Magazine A*, 64(1):137–150, 1991. doi: [10.1080/01418619108206131](https://doi.org/10.1080/01418619108206131).
- [7] N. M. Rosengaard and H. L. Skriver. *Ab initio* study of antiphase boundaries and stacking faults in  $\text{L1}_2$  and  $\text{DO}_{22}$  compounds. *Physical Review B*, 50(7):4848, 1994. doi: [10.1103/PhysRevB.50.4848](https://doi.org/10.1103/PhysRevB.50.4848).
- [8] O. N. Mryasov, Y. N. Gornostyrev, M. Van Schilfgaarde, and A. J. Freeman. Superdislocation core structure in  $\text{L1}_2$   $\text{Ni}_3\text{Al}$ ,  $\text{Ni}_3\text{Ge}$  and  $\text{Fe}_3\text{Ge}$ : Peierls–Nabarro analysis starting from *ab-initio* GSF energetics calculations. *Acta Materialia*, 50(18):4545–4554, 2002. doi: [10.1016/S1359-6454\(02\)00282-3](https://doi.org/10.1016/S1359-6454(02)00282-3).

- [9] X. X. Yu and C. Y. Wang. Effect of alloying element on dislocation cross-slip in  $\gamma'$ -Ni<sub>3</sub>Al: a first-principles study. *Philosophical Magazine*, 92(32):4028–4039, 2012. doi: [10.1080/14786435.2012.700419](https://doi.org/10.1080/14786435.2012.700419).
- [10] L. Liu, X. Wu, R. Wang, W. Li, and Q. Liu. Stacking fault energy, yield stress anomaly, and twinnability of Ni<sub>3</sub>Al: A first principles study. *Chinese Physics B*, 24(7):077102, 2015. doi: [10.1088/1674-1056/24/7/077102](https://doi.org/10.1088/1674-1056/24/7/077102).
- [11] Y. Rao, T. M. Smith, M. J. Mills, and M. Ghazisaeidi. Segregation of alloying elements to planar faults in  $\gamma'$ -Ni<sub>3</sub>Al. *Acta Materialia*, 148:173–184, 2018. doi: [10.1016/j.actamat.2018.01.055](https://doi.org/10.1016/j.actamat.2018.01.055).
- [12] Y. Mishin. Atomistic modeling of the  $\gamma$  and  $\gamma'$ -phases of the Ni–Al system. *Acta Materialia*, 52(6):1451–1467, 2004. doi: [10.1016/j.actamat.2003.11.026](https://doi.org/10.1016/j.actamat.2003.11.026).
- [13] S. P. Chen, D. J. Srolovitz, and A. F. Voter. Computer simulation on surfaces and [001] symmetric tilt grain boundaries in Ni, Al, and Ni<sub>3</sub>Al. *Journal of Materials Research*, 4(1):62–77, 1989. doi: [10.1557/JMR.1989.0062](https://doi.org/10.1557/JMR.1989.0062).
- [14] J. P. Du, C. Y. Wang, and T. Yu. Construction and application of multi-element EAM potential (Ni–Al–Re) in  $\gamma/\gamma'$  Ni-based single crystal superalloys. *Modelling and Simulation in Materials Science and Engineering*, 21(1):015007, 2012. doi: [10.1088/0965-0393/21/1/015007](https://doi.org/10.1088/0965-0393/21/1/015007).
